# Supplementary material for: Robust Active Site Design of Single Atom Catalysts for Electrochemical Ammonia Synthesis
Source: arXiv:2007.10318 source file (2020-07-15)
Supplement: Supplementary file 1 [file SI.pdf]

# Supporting Information for Robust Active Site Design of Single Atom Catalysts for Electrochemical Ammonia Synthesis

Lance Kavalsky and Venkatasubramanian Viswanathan*

*Department of Mechanical Engineering, Carnegie Mellon University, Pittsburgh, Pennsylvania 15213, USA*

E-mail: venkvis@cmu.edu

# Generation of the Probabilistic Activity Volcanoes

In this work we investigate scaling among the reaction energies of the NRR intermediates NNH*, $NH_2$*, and N*. From conducting an ordinary least squares fit on the energies of each member XC in the ensemble, a distribution of fitting parameters is obtained. This distribution provides another perspective of uncertainty by studying the stability of these scaling relationships towards functional selection. Using this ensemble of parameters allows for propagation of the uncertainty to generate an ensemble of activity volcanoes. Of the 2000 XC functionals in the ensemble, 19 are deemed unphysical because the slopes are such that an activity maximum did not occur. This approach is then utilized to generate a probabilistic activity volcano in terms of a conditional probability. This quantity describes the probability of the limiting potential $\mathrm{U_L}$ taking on a specific value given a single descriptor (in this case $\langle \Delta G_{\mathrm{NNH}^*} \rangle$). For notational convenience, we will represent the descriptor $\langle \Delta G_{\mathrm{NNH}^*} \rangle$ as $G$. Calculation of this conditional probability proceeds similarly to our previously outlined procedure but with relaxed scaling slope constraints.[1] First, for a given descriptor value and volcano in the ensemble there is an associated uncertainty, and we treat it as a gaussian distribution:

$$p_G(x|\mu = G, \sigma^2_{\mathrm{NNH}}) = \frac{1}{\sqrt{2\pi\sigma^2_{\mathrm{NNH}}}} \exp\left(\frac{-(x-\mu)^2}{2\sigma^2_{\mathrm{NNH}}}\right) \tag{S1}$$

where x is in the descriptor domain and $\sigma^2_{\mathrm{NNH}}$ is the variance of the combined $\Delta G_{\mathrm{NNH}^*}$ distribution. For the $i$-th volcano in the ensemble, we can calculate the probability for a specific limiting potential value given $G$ as a summation of all points on the volcano corresponding to that potential:

$$\hat{p}_i(\mathrm{U_L}|G) = \int_{-\infty}^{\infty} p_G(x|\mu = G, \sigma^2_{\mathrm{NNH}})\, \delta\left(f(x) - \mathrm{U_L}\right)\, \mathrm{d}x \tag{S2}$$

where $f(x)$ is an oracle function that maps the descriptor space to limiting potential space. More explicitly, this oracle function takes the form:

$$U_L = f(G) = -\frac{1}{e}\min(G, \Delta G_{2NH_3} - m^{(i)}G - b^{(i)}) \tag{S3}$$

which is just Eq. 13 from the main manuscript. Notice the $i$ superscripts for the scaling slope and intercept as these values are pulled from the scaling ensemble, and thus $N_{ens}$ different oracle functions emerge. For each ensemble member, the dirac delta function in Eq. S2 will extract two points in descriptor space, one for each leg of the $i$-th volcano. Normalization for a given descriptor value is then done via:

$$p_i(U_L|G) = \frac{\hat{p}_i(U_L|G)}{\int_{-\infty}^{U_L^{max}} \hat{p}_i(U_L|G)\, dU_L} \tag{S4}$$

Thus for every relation in the scaling ensemble, a different $p_i(U_L|G)$ emerges, with the average giving $p(U_L|G)$. To obtain the full probabilistic contour, we iterate over $G$ and then calculate $p(U_L|G)$ for each $U_L$ in a specified domain.

## $\Delta E_{\mathrm{NNH}^*}$ and $\Delta E_{\mathrm{H}^*}$ BEEF-vdW Ensembles

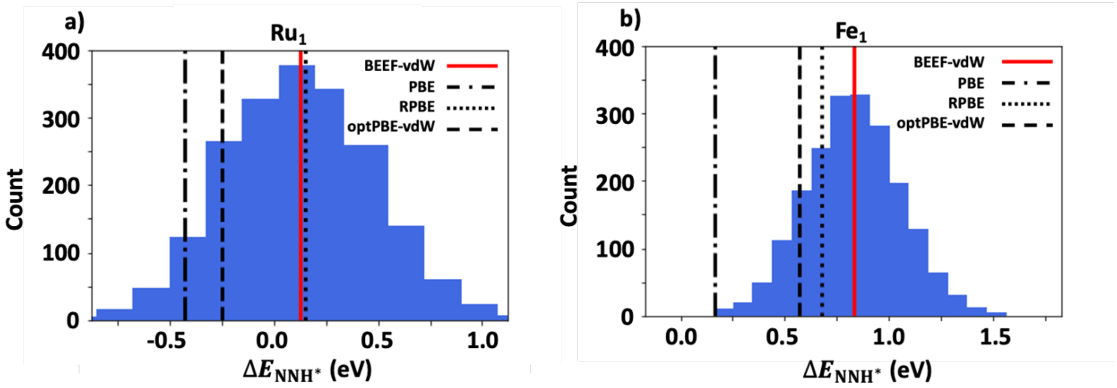


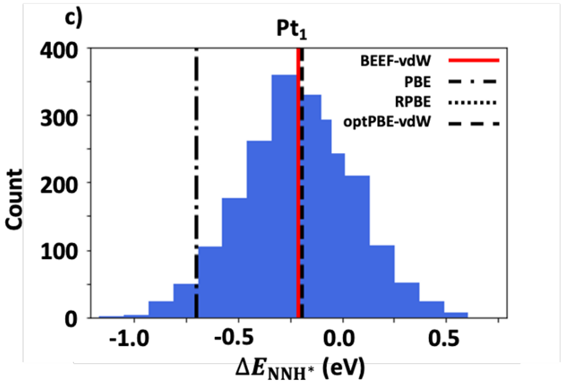


d)

| NNH* | $Ru_1$ | $Fe_1$ | $Pt_1$ |
|---|---|---|---|
| Skewness | 0.03 | 0.04 | -0.04 |
| Kurtosis | 3.09 | 2.91 | 2.94 |

Figure S1: Ensembles obtained from the BEEF-vdW XC for formation of NNH* on a) $Ru_1$, b) $Fe_1$, and $Pt_1$. d) Skewness and Kurtosis values for each of the ensembles. A normal distribution has a skewness of 0 and kurtosis of 3, thus indicating that these systems can be treated as normal

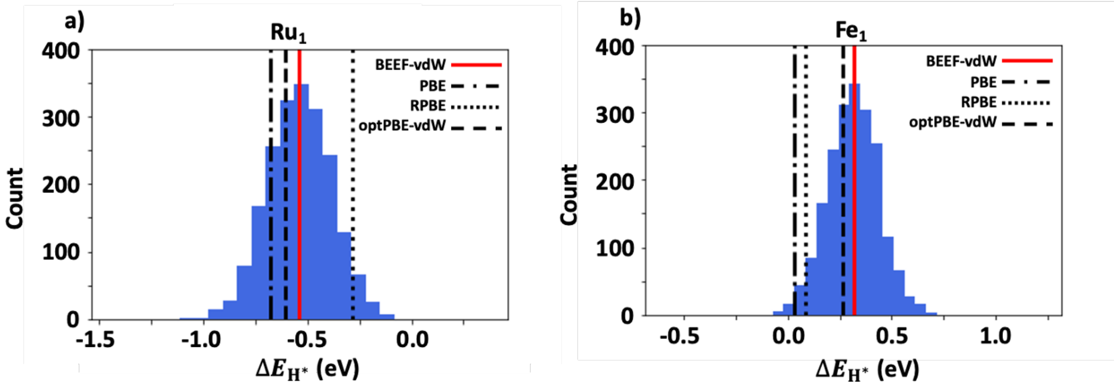


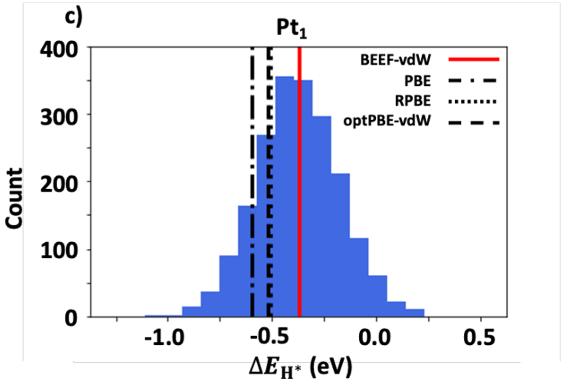


d)

| H* | $Ru_1$ | $Fe_1$ | $Pt_1$ |
|---|---|---|---|
| Skewness | -0.05 | 0.00 | 0.02 |
| Kurtosis | 2.91 | 3.02 | 2.99 |

Figure S2: Ensembles obtained from the BEEF-vdW XC for formation of H* on a) $Ru_1$, b) $Fe_1$, and $Pt_1$. d) Skewness and Kurtosis values for each of the ensembles. A normal distribution has a skewness of 0 and kurtosis of 3, thus indicating that these systems can be treated as normal

## Additional Free Energy Diagrams

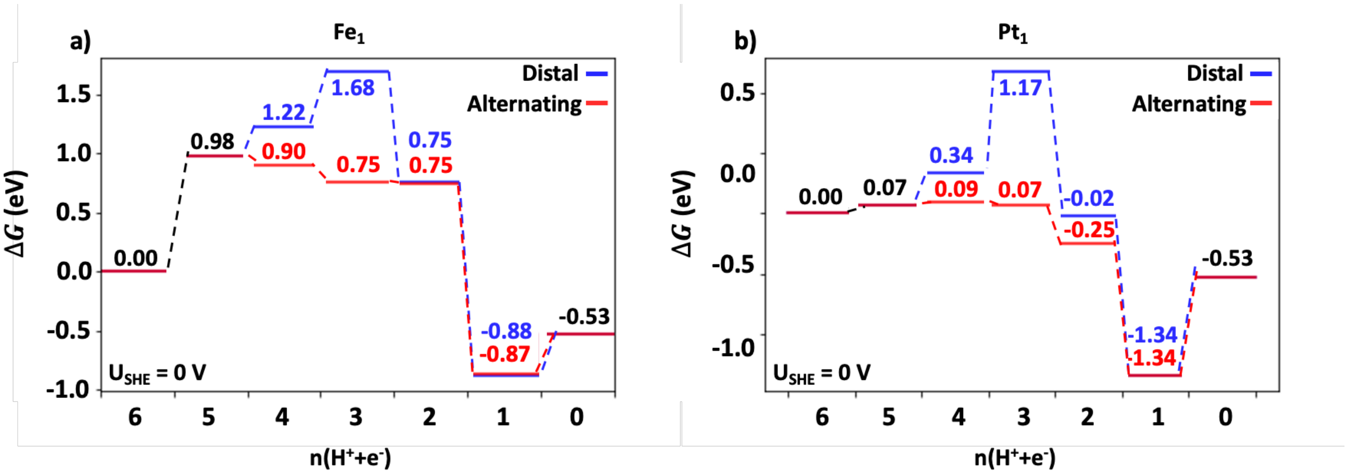


Figure S3: Free Energy diagrams for both the distal and alternating mechanisms on a) $Fe_1$ and b) $Pt_1$

## Additional Scaling Figures

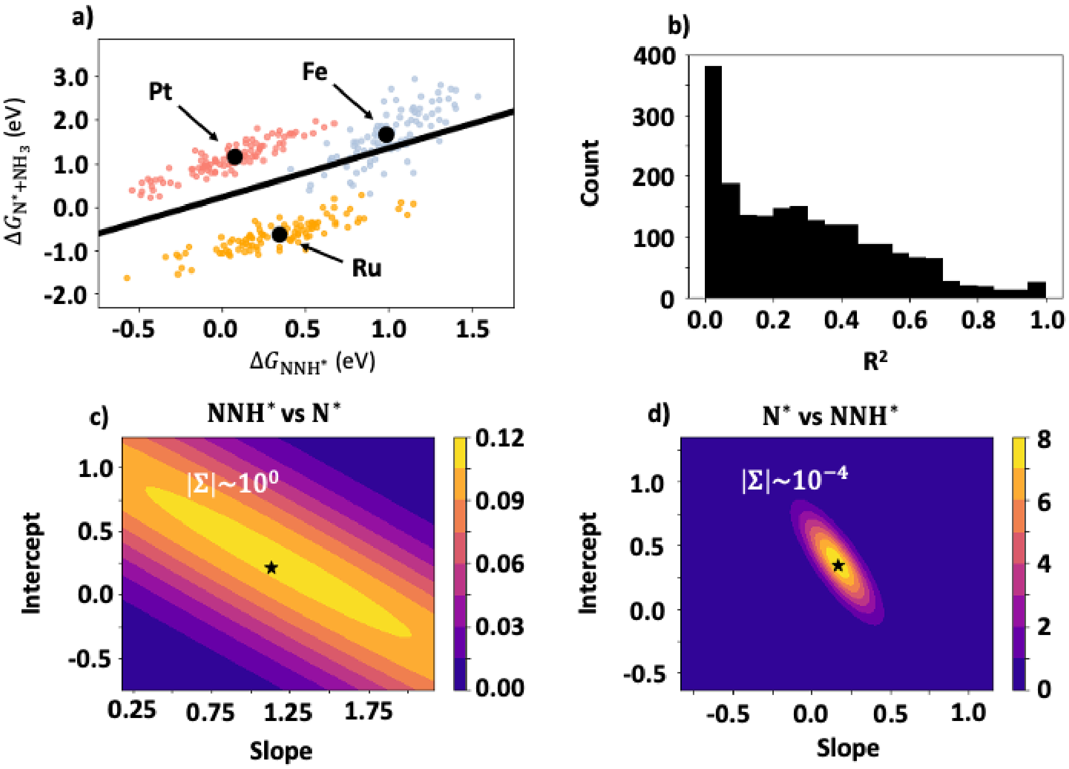


Figure S4: a) Scaling Relationship of $\Delta G_{\mathrm{NNH}^*}$ and $\Delta G_{\mathrm{N}^*}$. Black dots are the optimal BEEF-vdW values, with the solid black line the corresponding linear fit. The red, orange, and blue dots correspond to a sampling of 100 XC functionals from the BEEF-vdW ensemble for $Pt_1$, $Ru_1$, and $Fe_1$, respectively. b) Distribution of correlation coefficients for each of the scaling relation fits in the ensemble. Probability density distribution in parameter space for when c) $\Delta G_{\mathrm{NNH}^*}$ and d) $\Delta G_{\mathrm{N}^*}$ are the descriptors. The black stars correspond to the parameters from the optimal BEEF-vdW fit

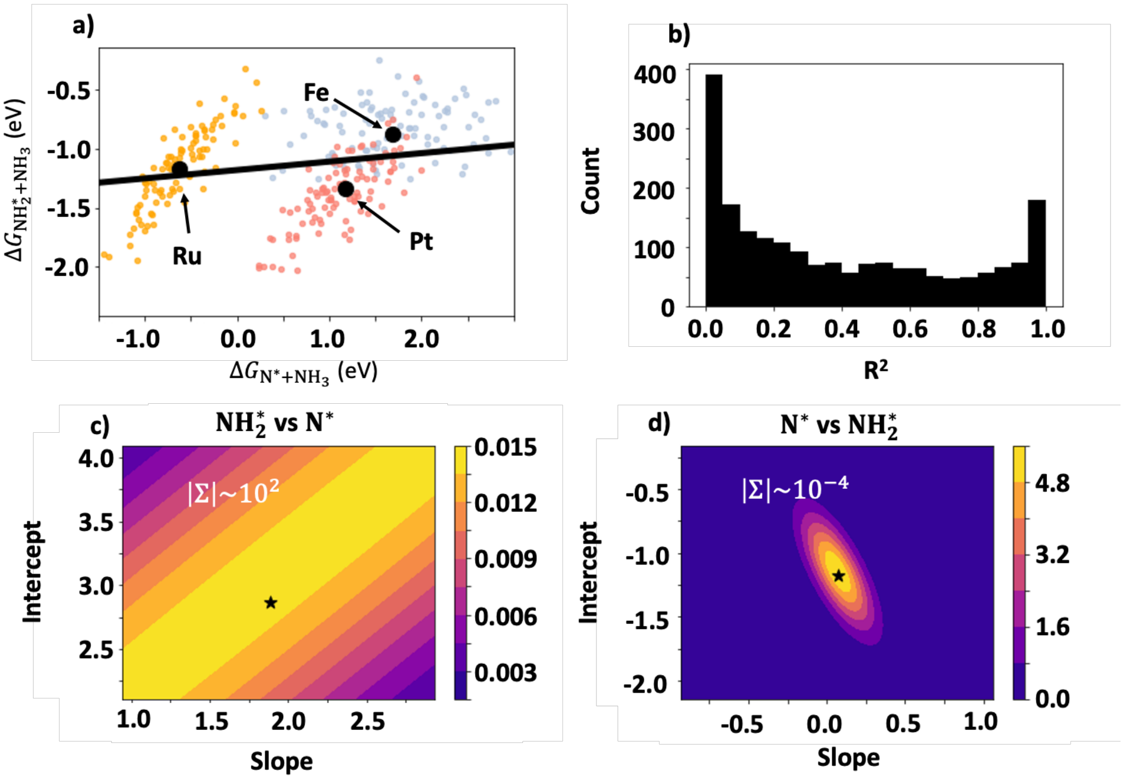


Figure S5: a) Scaling Relationship of $\Delta G_{NH_2^*}$ and $\Delta G_{N^*}$. Black dots are the optimal BEEF-vdW values, with the solid black line the corresponding linear fit. The red, orange, and blue dots correspond to a sampling of 100 XC functionals from the BEEF-vdW ensemble for $Pt_1$, $Ru_1$, and $Fe_1$, respectively. b) Distribution of correlation coefficients for each of the scaling relation fits in the ensemble. Probability density distribution in parameter space for when c) $\Delta G_{NH_2^*}$ and d) $\Delta G_{N^*}$ are the descriptors. The black stars correspond to the parameters from the optimal BEEF-vdW fit

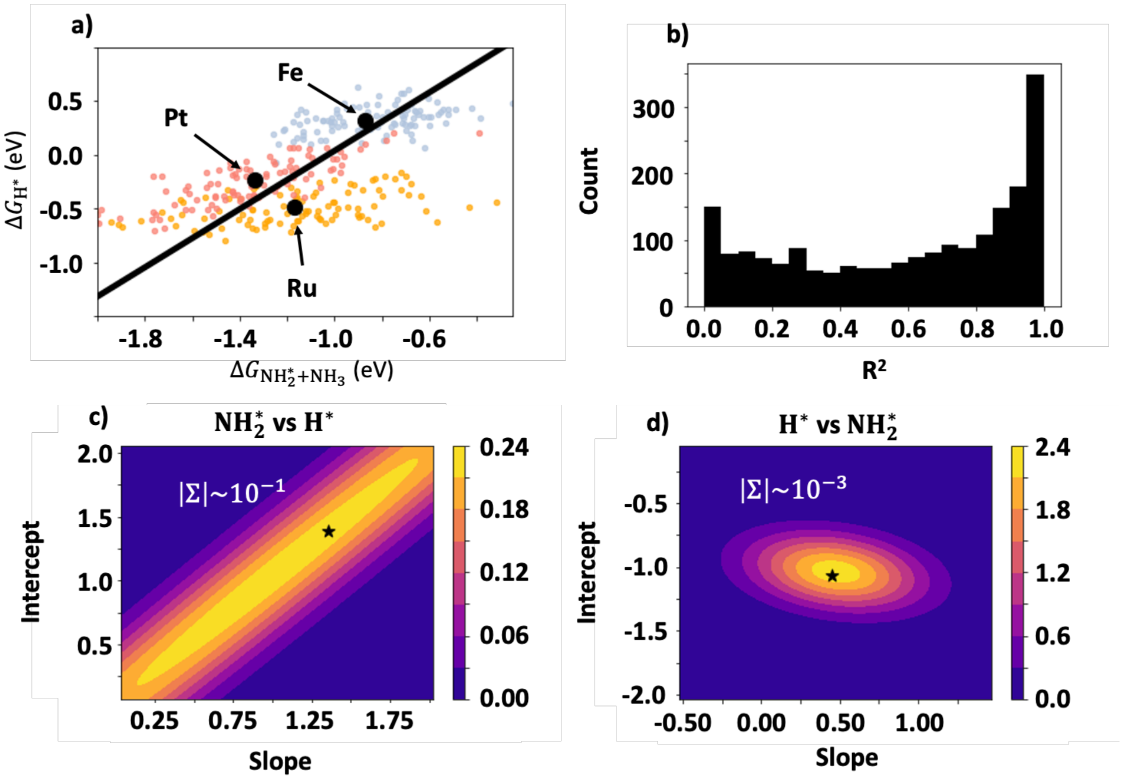


Figure S6: a) Scaling Relationship of $\Delta G_{\mathrm{NH}_2^*+\mathrm{NH}_3}$ and $\Delta G_{\mathrm{H}^*}$. Black dots are the optimal BEEF-vdW values, with the solid black line the corresponding linear fit. The red, orange, and blue dots correspond to a sampling of 100 XC functionals from the BEEF-vdW ensemble for $\mathrm{Pt}_1$, $\mathrm{Ru}_1$, and $\mathrm{Fe}_1$, respectively. b) Distribution of correlation coefficients for each of the scaling relation fits in the ensemble. Probability density distribution in parameter space for when c) $\Delta G_{\mathrm{NH}_2^*+\mathrm{NH}_3}$ and d) $\Delta G_{\mathrm{H}^*}$ are the descriptors. The black stars correspond to the parameters from the optimal BEEF-vdW fit

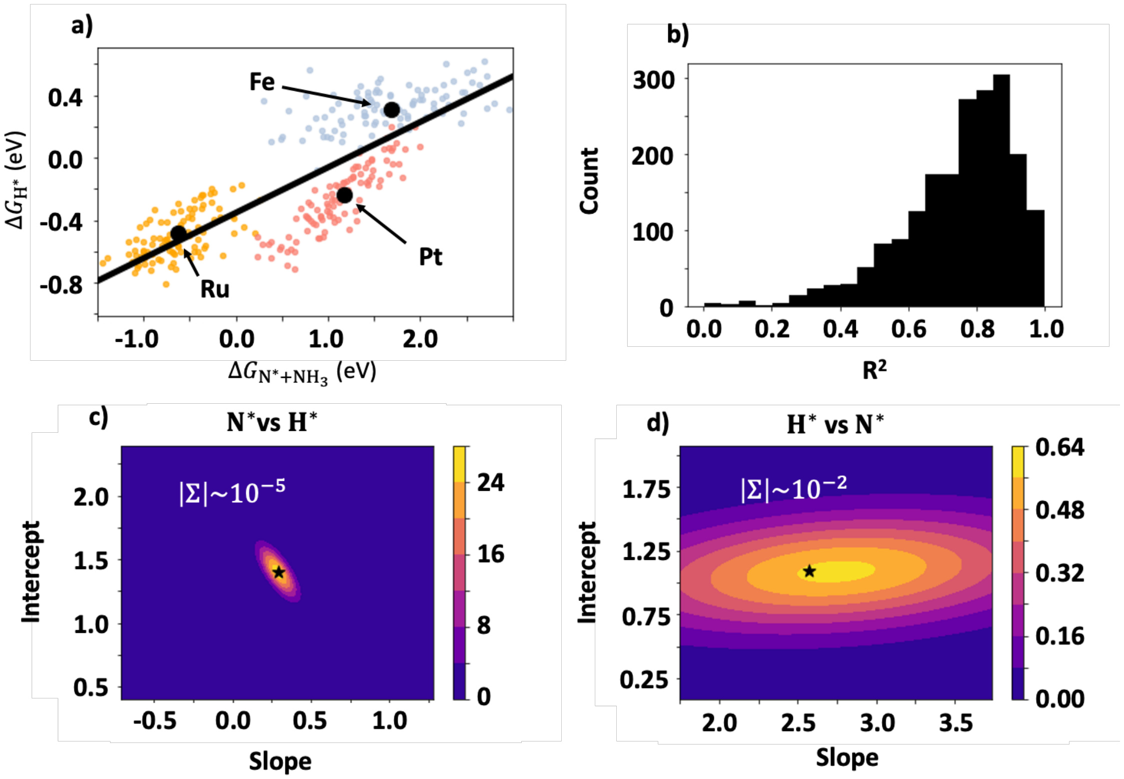


Figure S7: a) Scaling Relationship of $\Delta G_{N^*+NH_3}$ and $\Delta G_{H^*}$. Black dots are the optimal BEEF-vdW values, with the solid black line the corresponding linear fit. The red, orange, and blue dots correspond to a sampling of 100 XC functionals from the BEEF-vdW ensemble for $Pt_1$, $Ru_1$, and $Fe_1$, respectively. b) Distribution of correlation coefficients for each of the scaling relation fits in the ensemble. Probability density distribution in parameter space for when c) $\Delta G_{N^*+NH_3}$ and d) $\Delta G_{H^*}$ are the descriptors. The black stars correspond to the parameters from the optimal BEEF-vdW fit

## Probabilistic HER Volcano

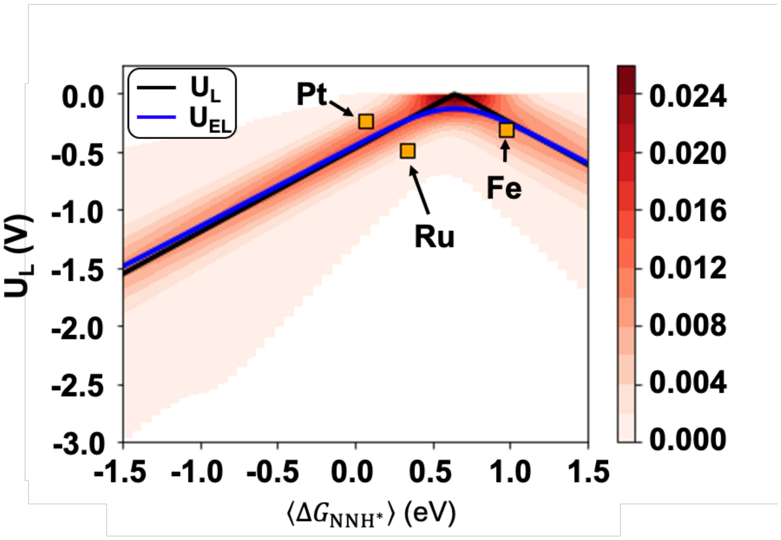


Figure S8: Probabilistic activity volcano for HER on these systems with the descriptor $\langle \Delta G_{\mathrm{NNH^*}} \rangle$. The solid black line is the limiting potential based on the optimal BEEF-vdW fitting parameters obtained from the sample. The solid blue line is the expected limiting potential which is the limiting potential weighted by the probability distribution. Orange squares are the BEEF-vdW optimal values

# References

(1) Krishnamurthy, D.; Sumaria, V.; Viswanathan, V. Maximal Predictability Approach for Identifying the Right Descriptors for Electrocatalytic Reactions. *Journal of Physical Chemistry Letters* **2018**, *9*, 588–595.
